# Supplementary material for: Scam Pandemic: How Attackers Exploit Public Fear through Phishing
Source: arXiv:2103.12843 source file (2021-03-23)
Supplement: Supplementary file 1 [file appendix.tex]

% \newpage
% \section{Appendix}
% Examples of phishing websites that exploit the COVID-19 pandemic.
% \textcolor{white}{
% Corona-themed phishing websites.
% }

\begin{figure}[h]
    \centering
    \includegraphics[width=.7\linewidth]{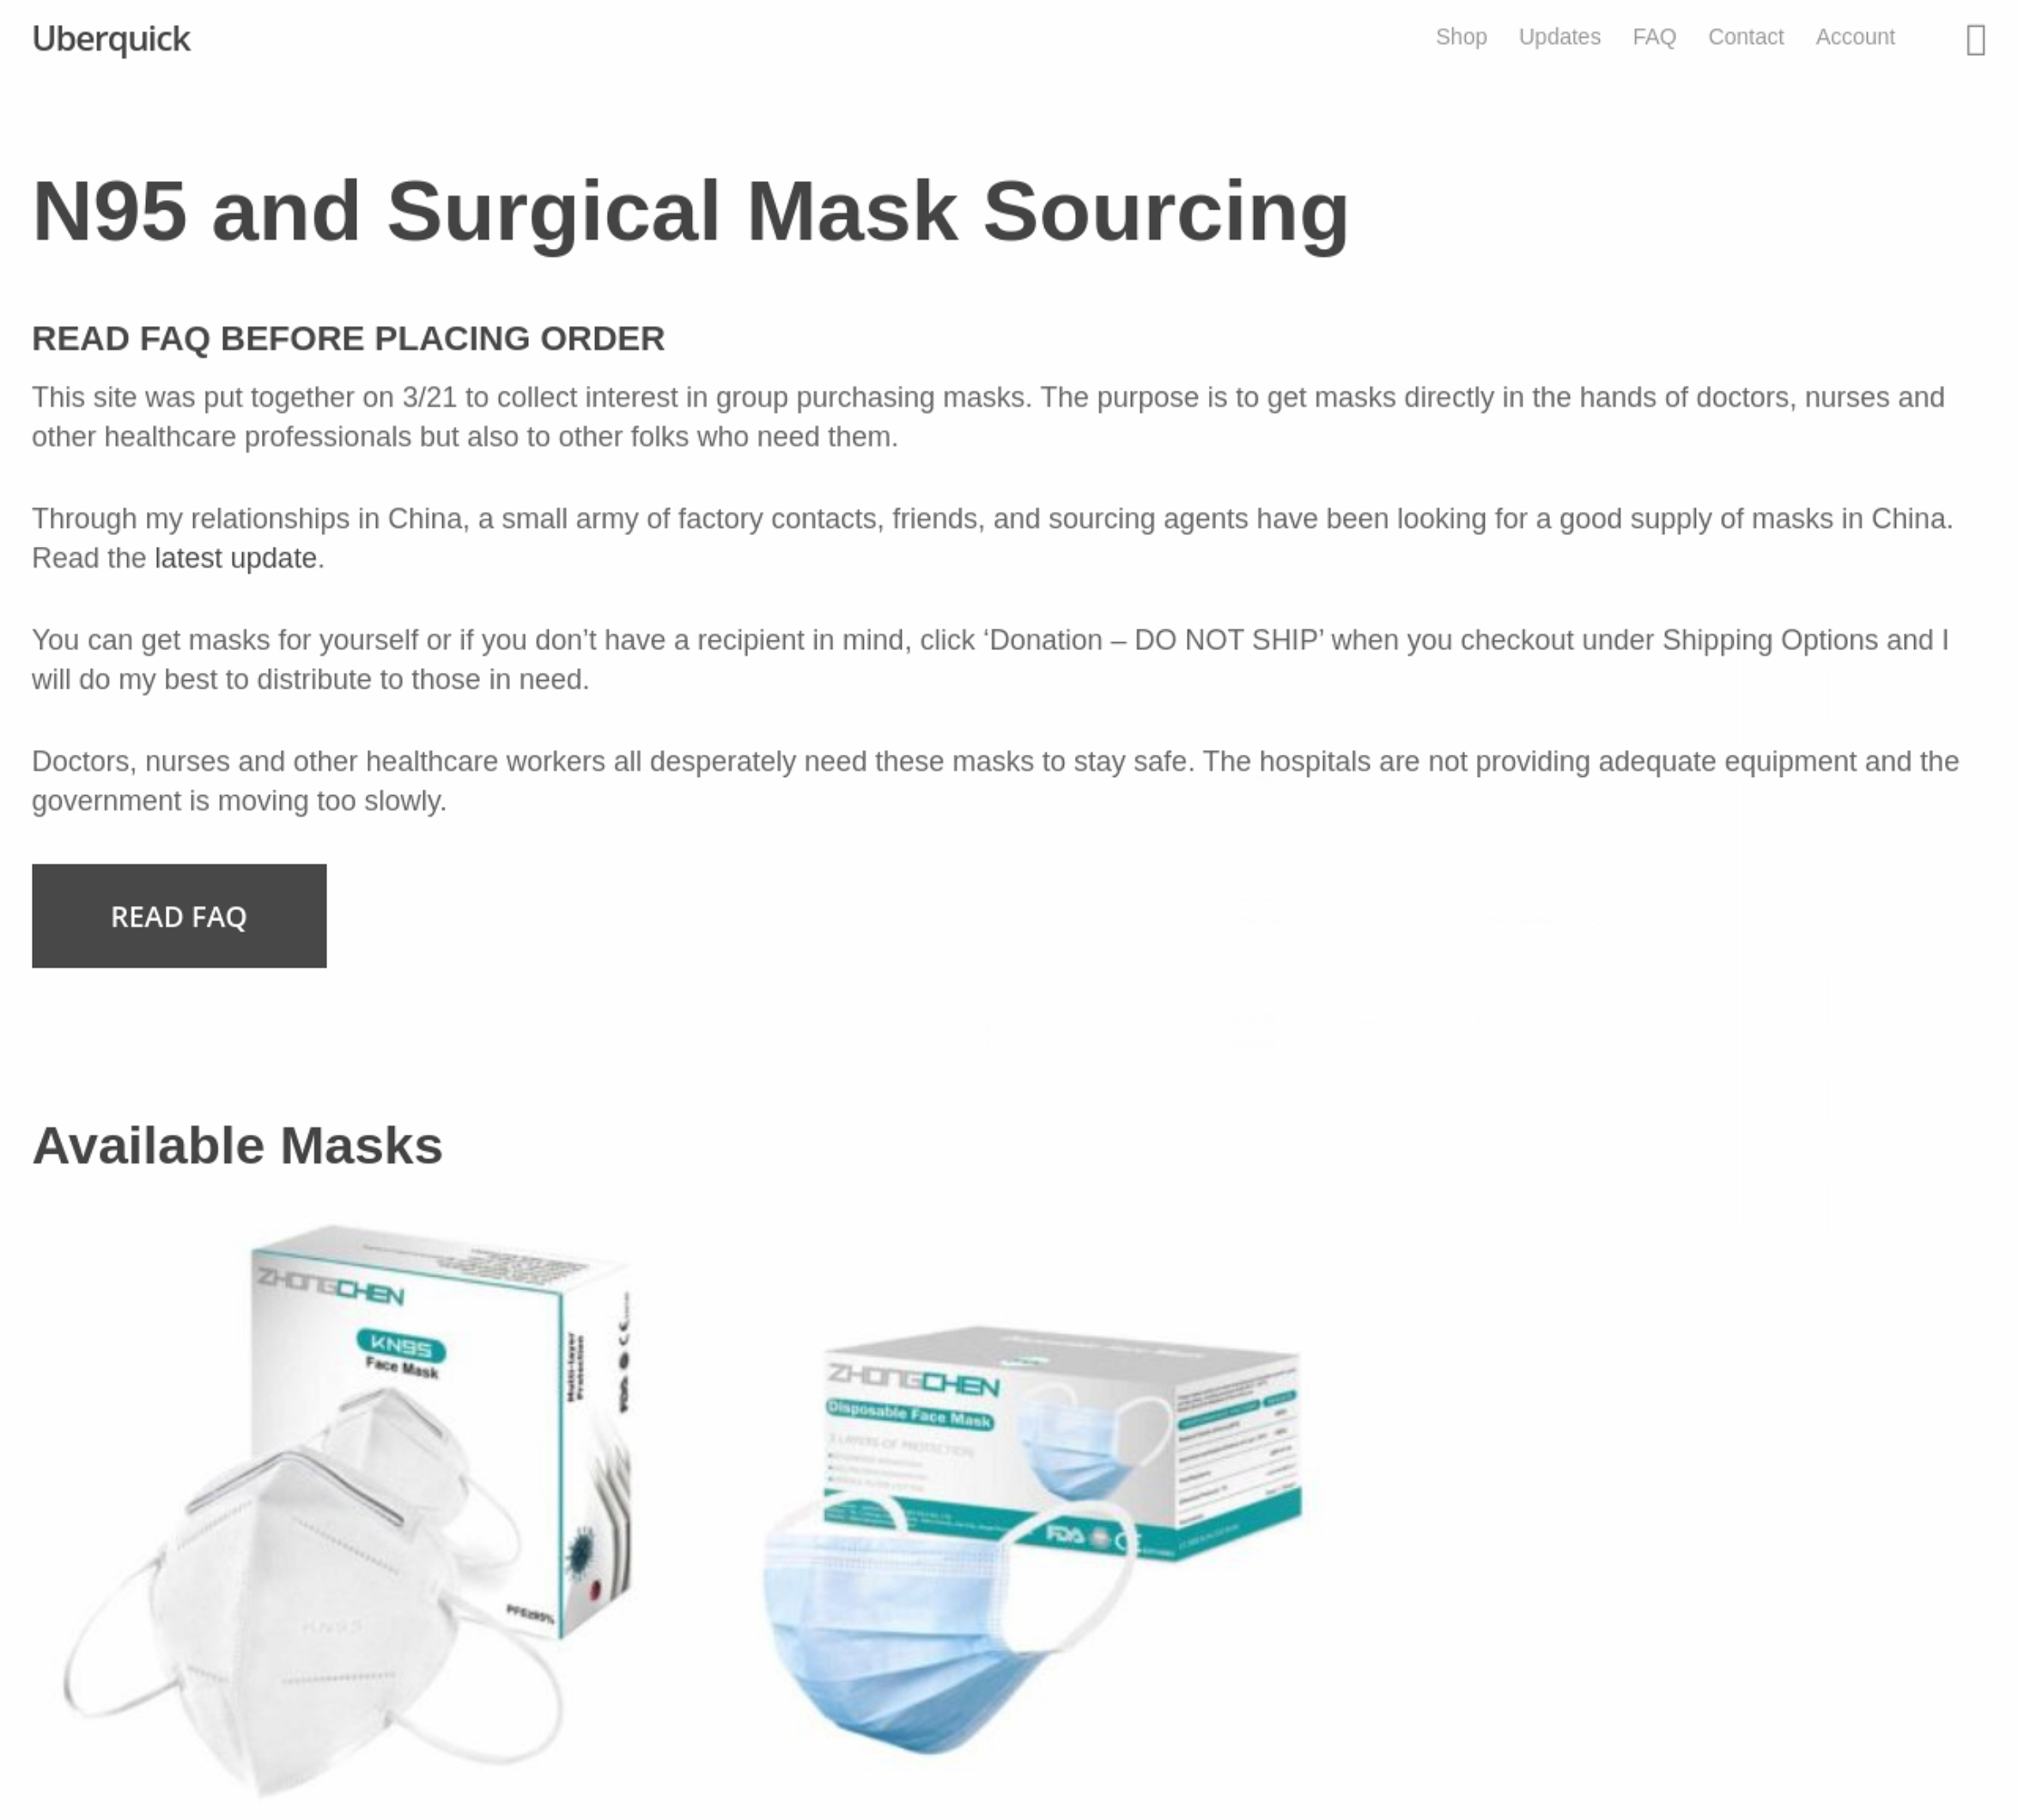}
    \caption{Fraudulent website selling PPE.}
    \label{fig:ppe_phishing}
\end{figure}

\begin{comment}
\begin{figure}[h]
    \centering
    \includegraphics[width=.7\linewidth]{figs/phishing_screenshot/followup.png}
    \caption{Fraudulent website following the pace of legitimate websites.}
    \label{fig:followup_phishing}
\end{figure}
\end{comment}

\begin{figure}[h]
    \centering
    \begin{subfigure}{0.43\linewidth}
        \centering
            \includegraphics[width=\textwidth]{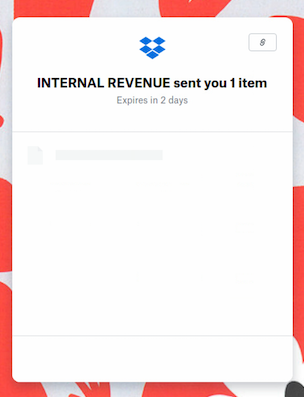}%
        \caption{Dropbox themed.}
        \label{fig:drobox}
    \end{subfigure}%          % end subfigure 1
    \hspace*{\fill}
    % \vspace*{8pt}
    % ~
    \begin{subfigure}{0.43\linewidth}
        \centering
            \includegraphics[width=\textwidth]{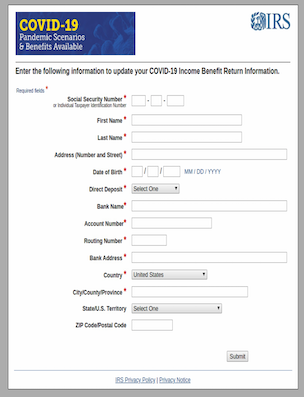}
        \caption{IRS themed.}
        \label{fig:irs}
    \end{subfigure}%          % end subfigure 2
    
    \caption{Phishing websites exploiting IRS.}
    \label{fig:irs_phishing}
\end{figure}

\begin{figure}[h]
    \centering
    \includegraphics[width=.7\linewidth]{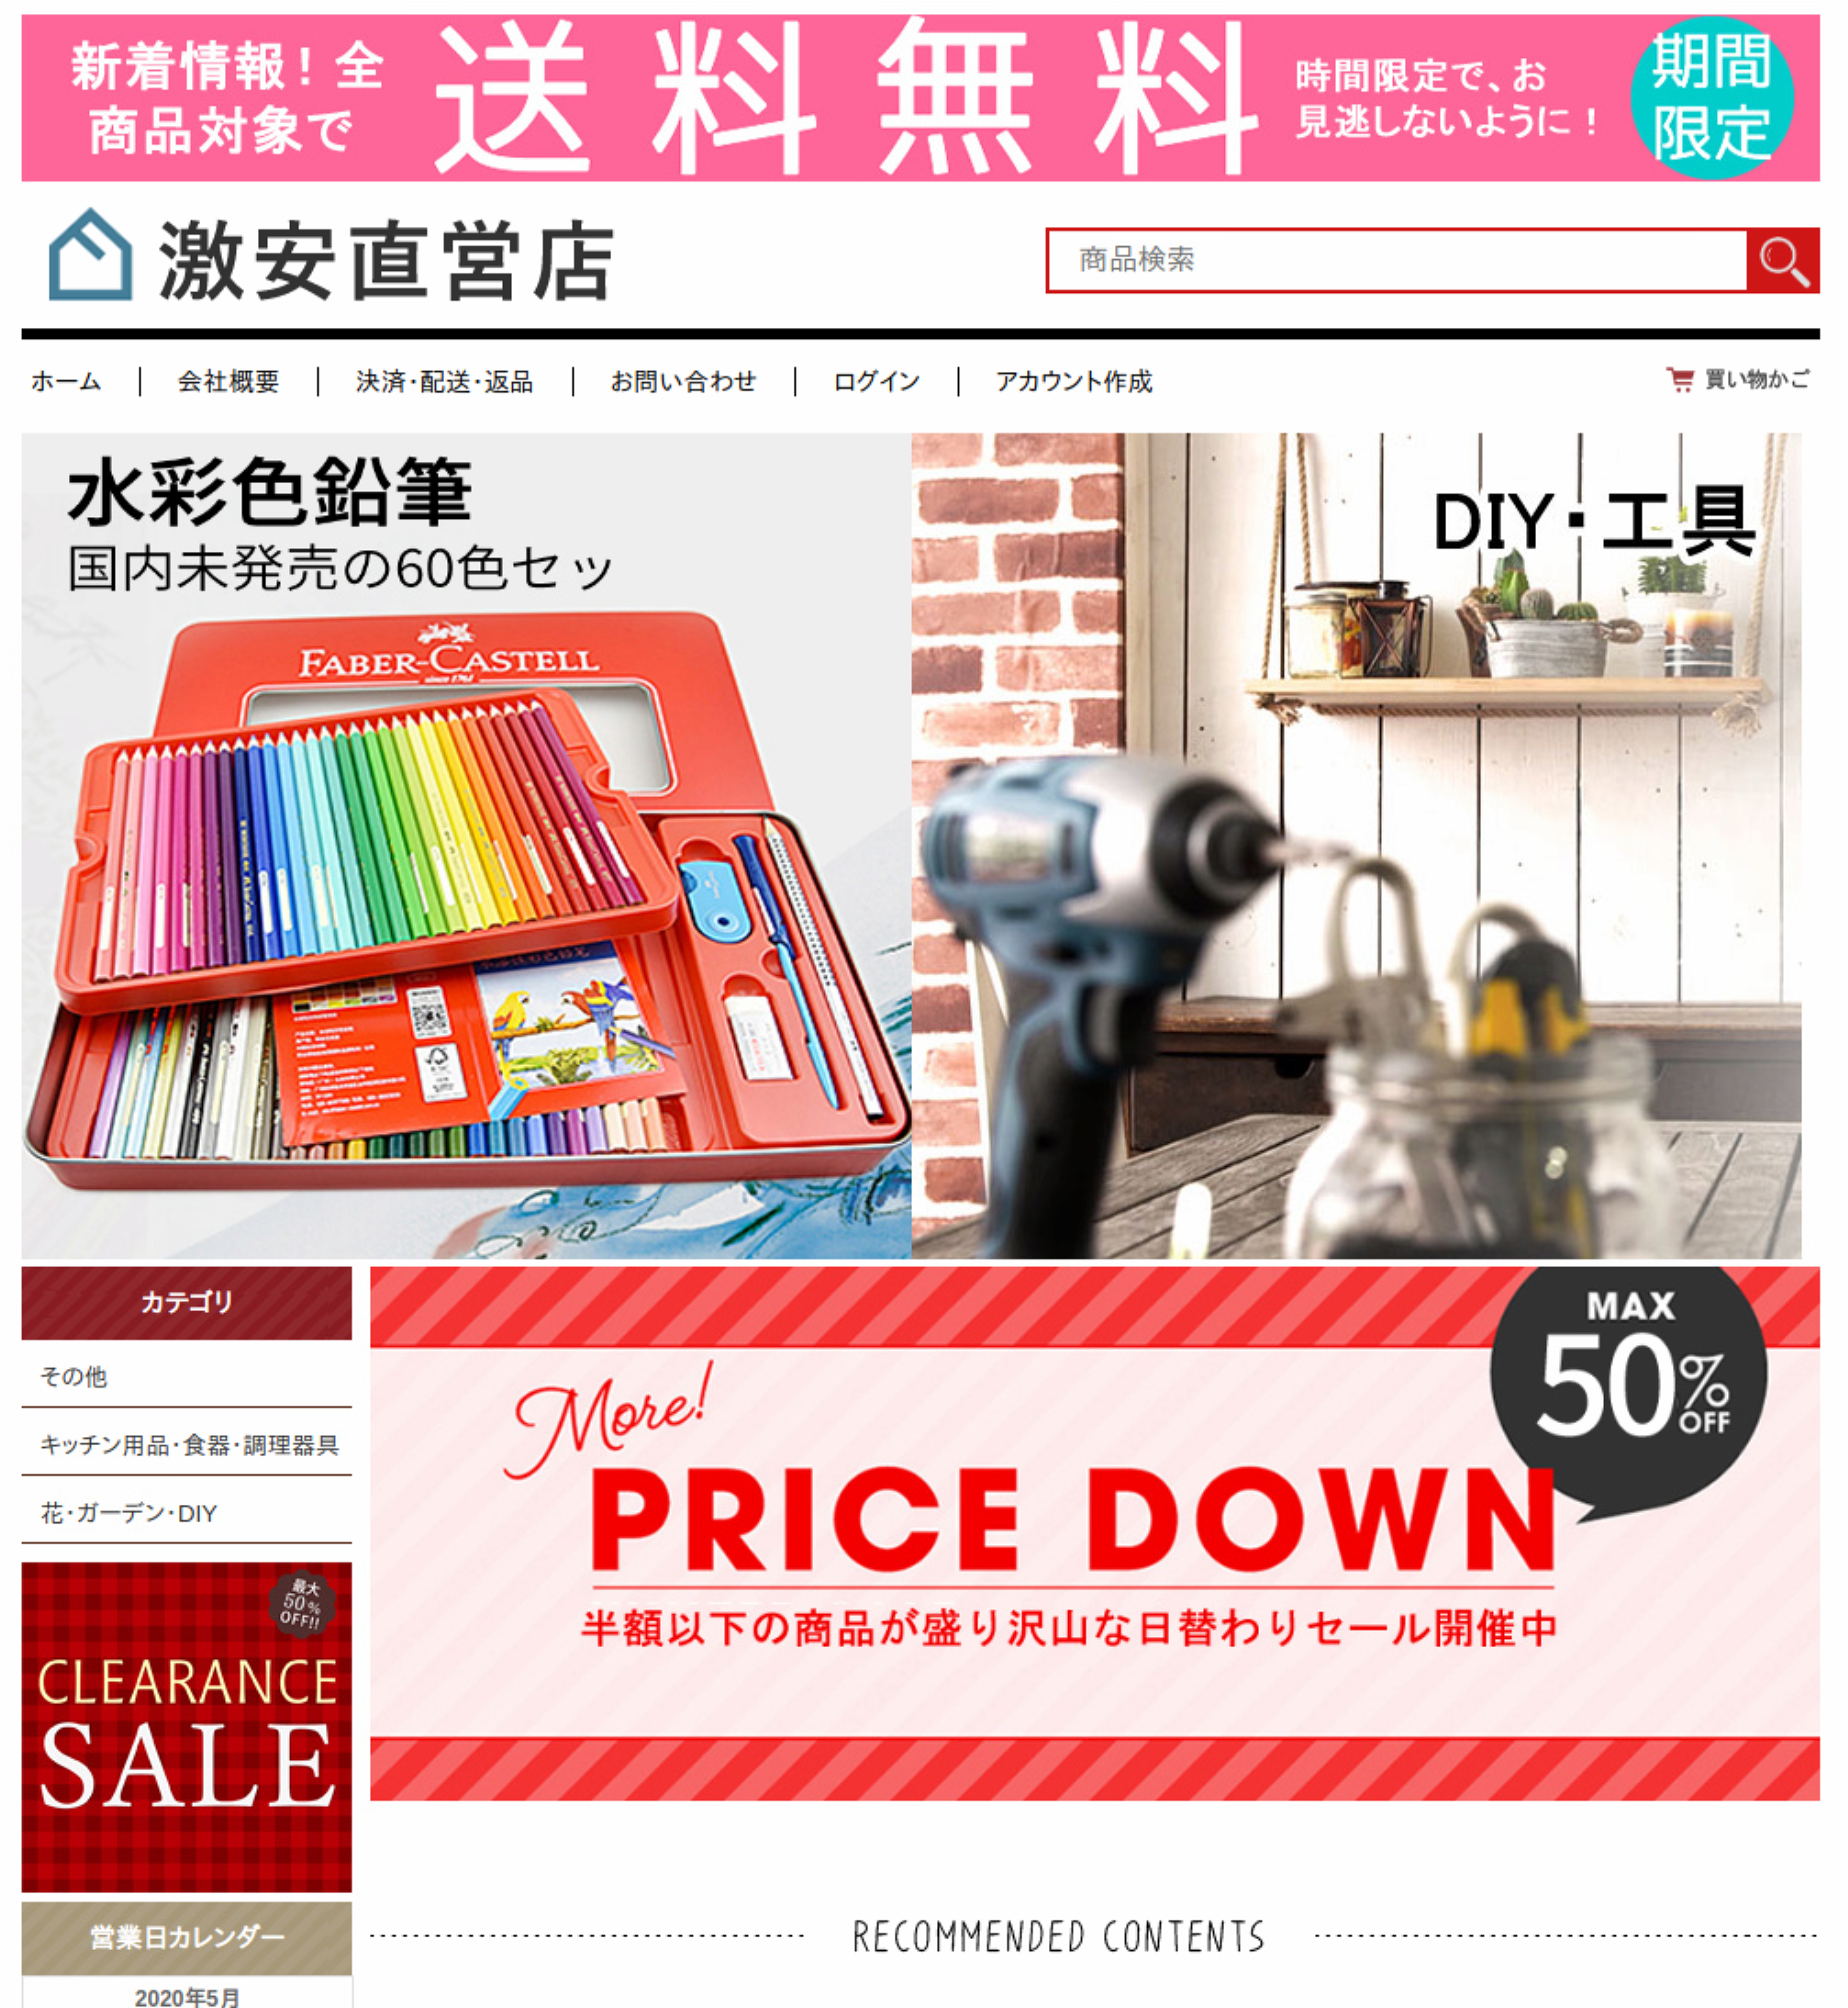}
    \caption{Free shipping fraudulent store.}
    \label{fig:freeshipping_phishing}
\end{figure}
